# Supplementary material for: Composable Interventions for Language Models
Source: arXiv:2407.06483 source file (2025-03-16)
Supplement: Supplementary file 1 [file token_changes.tex]

\subsection{Interpreting intervention interactions}

\begin{figure*}[!htpb]
    \centering
    \includegraphics[width=\linewidth]{figures/logits.pdf}
    \caption{Tokens for Llama-2 prompted with ``The next summer Olympics will be held in''. The correct answer ``Paris'' is shown in red. Editing successfully increases the scale of Paris, though compression shrinks it again. Compression maintains similar tokens, though hinders editing success. Blank token names are special characters.}
    \label{fig:logits}
\end{figure*}

% Visuals
We finally conduct a simple case study to visually investigate how logits change according to different intervention orders.
Specifically, we study predicted logits from the LM before and after each intervention in isolation and after their composition.
We pick one real edit about the location of the next summer Olympic games. Before editing, Llama-2 consistently predicts ``The next summer Olympics will be held in'' $\to$ ``Tokyo''. But the correct answer is ``Paris''. As shown in Figure \ref{fig:logits} in Appendix \ref{apdx:interpretation}, we then plot Llama-2's top-30 predicted logits and observe that ``Tokyo'' is indeed the largest, while the correct ``Paris'' (in red) is the third largest.
We then edit the model to confidently 
